# Supplementary material for: Learning Part Motion of Articulated Objects Using Spatially Continuous Neural Implicit Representations
Source: arXiv:2311.12407 source file (2023-11-21)
Supplement: Supplementary file 1 [file supp.tex]

\appendix

\tableofcontents

\section{More Details in the Main Paper}
\subsection{Network Details}
We sample $N=8192$ points for the input point clouds, using PointNet++~\cite{qi2017pointnetplusplus} which subsamples them to $N'=128$ points with a $d=256$ dimension feature on each point.
After the attention layer, we feed subsampled points to PointNet++ decoders that output dense point features aligned with input point clouds, with a 64 dimension feature on each point. 
The resolution and feature dimensions of the 3D grid output by 3D-UNet are $32\times32\times32$ and 64.
The \textbf{Pose Encoder} we use to encode part poses is a three-layer MLP, with output dimension of each layer to be $64, 128$, and $256$. All layers use the ReLU function as activation.

\subsection{Data Details}
We use the large-scale PartNet-Mobility dataset for its diversity in object articulations and rich geometry details of objects. 
We select 236 different objects over 8 categories in total and collect 100 instances with different part poses for each object. The proportion between instances for training and testing is approximately 7: 1.
% We collect novel instances from both seen objects and unseen objects during training for the test set, the proportion between instances from seen objects and unseen objects is approximately 1: 5 which differs depending on object categories.

\subsection{Baseline Implementation Details}
We modify each baseline to fit our settings, and thus we can have fair comparisons.

For A-SDF~\cite{mu2021sdf}, the original version of it performs badly due to its simple network architectures. % and the absence of the inference step. 
Therefore, we use the same PointNet++ encoder and \textbf{Part Encoder} as in our method to be the feature extractor of A-SDF, while not providing the 3D-UNet to project the points into a 3D feature grid. 
% Instead of using the feature of the whole point cloud to directly generate the object with the new part pose 
% We find that decoding each point
Then, we generate the point cloud with part pose $\phi_3$ directly using the extracted per-point feature, without our proposed per-point transformation matrices.
% We directly pass down the dense point features output by the PointNet++ module to the \textbf{Part Motion decoder}. In the \textbf{Part Motion Generation} step, we decode the point feature into point cloud under pose $\phi_3$ directly instead of generating the per-point transformation matrices by modifying the output dimensions of the \textbf{Part Motion Decoder} from 16 which is the dimension for transformation matrix, to 3 which presents the \textbf{xyz} coordinates of the output point cloud.

For another baseline, Ditto~\cite{jiang2022ditto}, we do not provide occupancy and articulation annotations, as we can fulfill the task without them.
We generate the point cloud with part pose $\phi_3$ directly using the extracted per-point feature, instead of using our proposed per-point transformation matrices.
% We implement it as generating the point cloud under pose $\phi_3$ directly without the per-point transformation matrices using the same method mentioned above. The other part of the modified version of Ditto is the same as ours.

\subsection{Further Explanations of Experiment Results}
In Figure~{4} of the main paper, among all the object categories, our method works significantly better than other methods in \textbf{Door} and \textbf{Microwave}. 

\begin{figure*}
    \centering % left bottom right top)
    \includegraphics[trim={100, 40, 100, 60}, clip, scale=0.45]{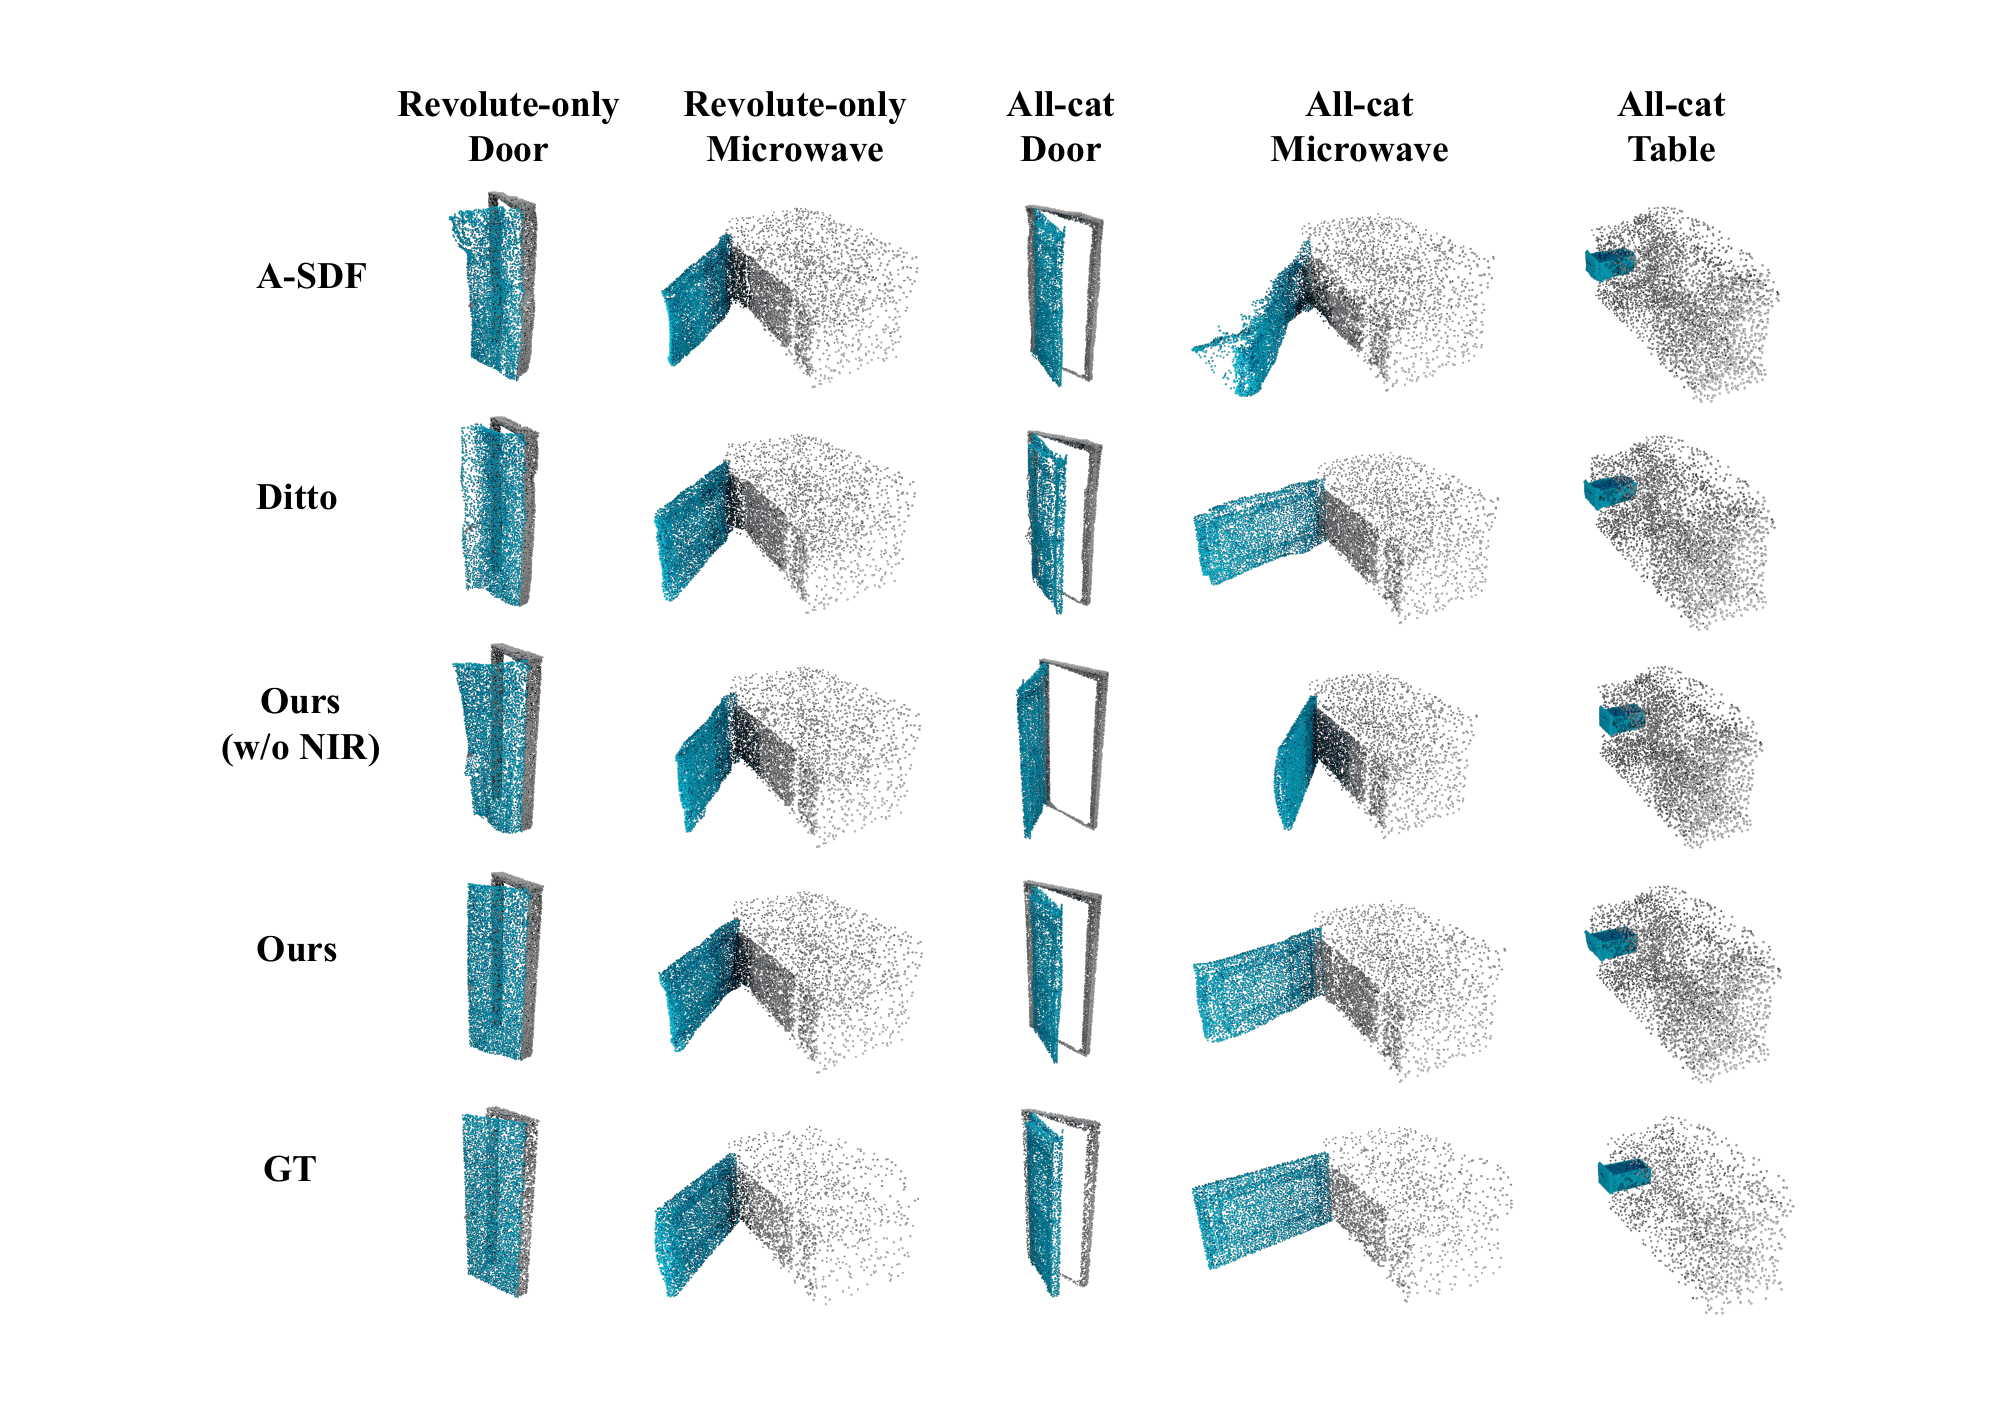}
    \vspace{4mm}
    \caption{
    \textbf{Visualization of multi-category experiment results.} 
    It is clear that our method outperforms other methods in (1) generating objects with smooth surfaces, (2) generating parts with accurate poses.
    }
    \label{fig:Multi_cat}
    \vspace{-2mm}
\end{figure*}

The reason is that, in our training data, these two categories have different joint orientations (\emph{e.g.}, clockwise and anti-clockwise orientations for doors) within them, and thus being more complicated than other object categories. Categories owning this feature are \textbf{Door} (4 directions), \textbf{Microwave} (2 directions), \textbf{Refrigerator} (2 directions), and \textbf{Scissors} (2 directions). We denote these categories as \textbf{Articulation-diverse} categories.

In Figure~{5} of the main paper, all methods perform better on the \textbf{Door-Laptop} setting than others, for the reason that the \textbf{Door} category is a \textbf{Articulation diverse} category with the most diverse joint orientations, so the model trained on \textbf{Door} is able to learn a more generic representation, and thus can easily generalize to other object categories.

\begin{table*}
  \centering
    \resizebox{\textwidth}{!}{
    \begin{tabular}{@{}lcccccccccc@{}}
    \toprule
    Category   & Laptop & Door & Refrigerator & Oven & Microwave & Stapler & Table & \\ \midrule \midrule 
    Number of instances    & 600 & 1200 & 1000 & 400 & 400 & 400 & 400 & \\ \bottomrule
    \end{tabular}
    }
  \vspace{4mm}
  \caption{\textbf{Data used in multi-category experiments.}}
  \vspace{-2mm}
  \label{multi_cat_data}
\end{table*}

\begin{table}[t]
\begin{minipage}{.48\textwidth}
  \centering
  \vspace{-5mm}
    \resizebox{\columnwidth}{!}{
    \begin{tabular}{@{}lcccccccccc@{}}
    \toprule
    Setting   & Revolute-only & All-cat & \\ \midrule \midrule
    A-SDF    & 2.4125 & 2.1318 & \\ \midrule
    Ditto    & 2.5901 & 2.8800 & \\ \midrule
    Ours w/o NIR & 3.0751 & 10.7618 & \\ \midrule
    Ours & \textbf{2.3945} & \textbf{2.1042} & \\ \bottomrule
    \end{tabular}
    }
  \vspace{3mm}
  \caption{\textbf{Earth Mover’s Distance (EMD) on articulated object generation in multi-category settings.} The articulation diversity complicates the task and thus forces the model to learn more generic representations.}
  \vspace{-5mm}
  \label{tab_interpolation}
\end{minipage}\hfill
\begin{minipage}{.48\textwidth}
  \centering
  \vspace{0mm}
    \resizebox{\columnwidth}{!}{
    \begin{tabular}{@{}lcccccccccc@{}}
    \toprule
    Setting   & Before tune & After tune & \\ \midrule \midrule 
    A-SDF    & 11.3914 & 2.7786 & \\ \midrule
    Ditto    & 12.3114 & 3.3318 & \\ \midrule
    Ours w/o NIR & 11.2056 & 14.9411 & \\ \midrule
    Ours & \textbf{10.7623} & \textbf{2.4877} & \\ \bottomrule
    \end{tabular}
    }
  \vspace{3mm}
  \caption{\textbf{EMD on articulated object generation in multi-category settings, model trained on Revolute-only categories and slightly tuned on Table.} Our method outperforms others.}
  \label{tab_multi_cat}
\end{minipage}
\end{table}

\section{Experiments on Multi-category Settings}

\subsection{Settings}
In the main paper, all models are trained in one object category.
Here, we show experiment results of models trained on multiple object categories, further demonstrating the generalization ability of our proposed method.
Specifically, we train our model in 7 object categories, with the number of sampled object instances with diverse part poses shown in Table~\ref{multi_cat_data}. 
This experiment is denoted as \textbf{All-cat}.

Additionally, to study our method's generalization ability from `revolute' joint to `prismatic' joint, we select all the 6 categories of objects with revolute joint for training, and test its generalization ability towards \textbf{Table} with prismatic joint.
This experiment is denoted as \textbf{Revolute-only}.
% We carry out experiments on multi-category settings to test the generalizability of our method. 
% We train the pipelines on both revolute-only data and the entire dataset, denoted as \textbf{Revolute-only} and \textbf{All-cat}.
% The data we used are listed in Table~\ref{multi_cat_data}. For \textbf{Revolute-only} we do not include the \textbf{Table} category while for \textbf{All-cat} we use all the data shown in Table~\ref{multi_cat_data}. 

\subsection{Object Generation with New Part poses}\label{subsec:totc}
\vspace{-1mm}
We evaluate our method by generating objects with new part poses, the same as in the main paper.
Table~\ref{tab_multi_cat} shows that our method outperforms others quantitatively.
Figure~\ref{fig:Multi_cat} shows that our method works better in generating (1) objects with smooth surfaces, (2) parts with accurate poses.

In this multi-category setting, the articulation diversity complicates the task and thus forces models to generically learn part motions of diverse articulations. The results show our proposed method learns more generic representations.

\begin{figure*}
    \centering % left bottom right top)
    \vspace{0mm}
    \includegraphics[trim={120, 280, 150, 30}, clip, scale=0.5]{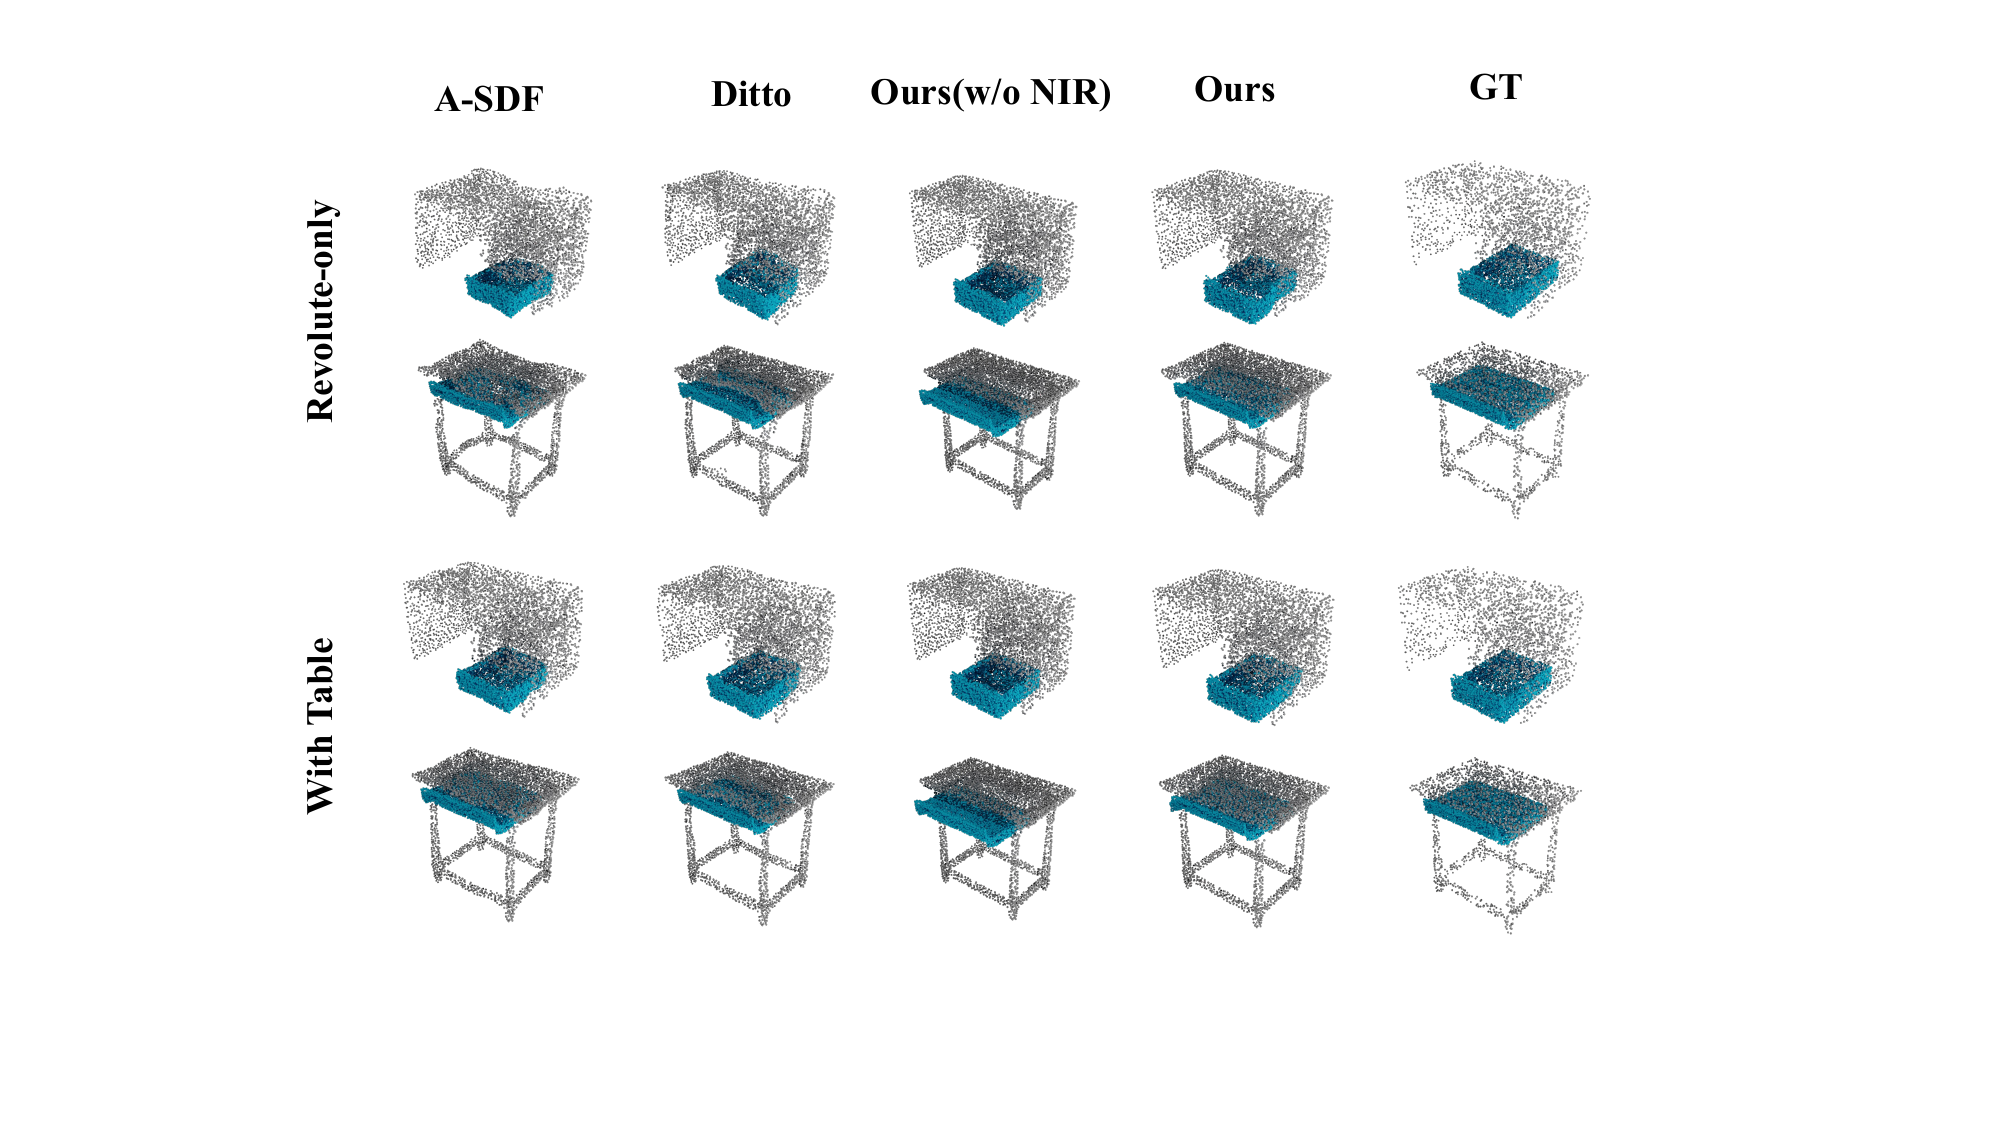}
    \vspace{4mm}
    \caption{
    \textbf{Visualization of tables generated by models trained under Revolute-only categories and slightly finetuned on the Table category.}
    Our method outperforms other methods in (1) generating objects with smooth surfaces, (2) generating parts with accurate poses.
    }
    \vspace{-3mm}
    \label{fig:tune_on_table}
\end{figure*}

% on instances from unseen objects on seen categories. Qualitative results are shown in Figure~\ref{fig:Multi_cat} and quantitative results are shown in Table~\ref{multi_cat}. 
% The qualitative results show that our method keeps the integrity of parts better and generates objects with smoother surfaces and fewer outliers than baseline methods and the ablated version, especially in face of the \textbf{Articulation diverse} categories we mentioned above where the task is more difficult. We found that the generation results ablated version of our method are usually the same as the input point cloud $I_1$, which shows that it tends to not move the input points at all. We attribute it to the way we train the transformation matrices which is to learn a residual of a matrix indicating zero scaling, rotation, and translation.

\subsection{Generalization from `Revolute' to 'Prismatic'}

\begin{wraptable}{l}{6.5cm}
  \centering
  \vspace{-4mm}
    \setlength{\tabcolsep}{1.2mm}
    
  \vspace{3mm}
  \caption{\textbf{EMD on articulated object generation in multi-category settings, model trained on Revolute-only categories and slightly tuned on Table.}}
  \vspace{-3mm}
  \label{tab_multi_cat}
\end{wraptable}

We train our model on \textbf{Revolute-only} categories, and slightly finetune it on \textbf{Table} category, to study our method's generalization ability from `revolute' joints to `prismatic' joints.
It is worth mentioning that, the finetuning only consumes \textbf{1/150} of the time for training.

Table~\ref{tab_multi_cat} shows that our method outperforms others, and Neural Implicit Representations (NIR) help a lot in our method's generalization ability. 
Figure~\ref{fig:tune_on_table} shows that our method successfully generates tables with new drawer poses, and clearly outperforms other methods in (1) generating objects with smooth surfaces, (2) generating parts with accurate poses.

% \begin{wraptable}{l}{6.5cm}
%   \centering
%   \vspace{-3mm}
%   % \setlength{\tabcolsep}{1.2mm}
%     \input{tabs/finetune.tex}
%   \vspace{4mm}
%   \caption{\textbf{Earth Mover’s Distance (EMD) on articulated object generation (in novel categories).} The results demonstrate that, after a short period of finetuning, our framework outperforms all other baselines and the ablated version in all novel categories.
%   % \textbf{Quantitative results on finetune} \yan{xxx}
%   }
%   % \vspace{-1mm}
%   \label{tab_quan_novel}
% \end{wraptable}
